# Supplementary material for: Incorporating Rich Social Interactions Into MDPs
Source: arXiv:2110.10298 source file (2022-02-07)
Supplement: Supplementary file 1 [file appendix.tex]

\section{Experiments}

The list of all 72 experimental scenarios  \footnote{Interactions for the experimental scenarios can be viewed at \url{https://social-interactions-mdp.github.io/scenarios}} varied across physical goals and social goals (in randomized order) for the two agents (yellow robot and red robot), \cref{tab:experiments}. Each scenario has agents as having either the same physical goal or different physical goals and one of 6 different social goals (cooperate, conflict, coercion, exchange or None) ($2*6*6=72$ scenarios).

\begin{longtable}[c]{@{}ccccc@{}}
\caption{An enumeration of all 72 scenarios for different configurations of physical and social goals of the robots.}
\label{tab:experiments}\\
Scenario Id & \multicolumn{2}{c}{Yellow Robot}    & \multicolumn{2}{c}{Red Robot}       \\
\cmidrule(lr){2-3}\cmidrule(lr){4-5}
\endfirsthead
    & Physical Goal & Social Goal & Physical Goal & Social Goal \\[2ex]
S1          & Tree         & None    & Construction Site & Cooperate  \\
S2          & Construction Site & None    & Tree         & Conflict   \\
S3          & Tree         & None    & Construction Site & Competiton \\
S4          & Tree         & None    & Construction Site & Coercion   \\
S5          & Construction Site & None    & Tree         & Exchange   \\
S6          & Tree         & None    & Construction Site & None    \\
S7          & Tree         & Cooperate  & Construction Site & Cooperate  \\
S8          & Construction Site & Cooperate  & Tree         & Conflict   \\
S9          & Tree         & Cooperate  & Construction Site & Competiton \\
S10         & Tree         & Cooperate  & Construction Site & Coercion   \\
S11         & Construction Site & Cooperate  & Tree         & Exchange   \\
S12         & Tree         & Cooperate  & Construction Site & None    \\
S13         & Construction Site & Conflict   & Tree         & Cooperate  \\
S14         & Construction Site & Conflict   & Tree         & Conflict   \\
S15         & Tree         & Conflict   & Construction Site & Competiton \\
S16         &              & Conflict   &              & Coercion   \\
S17         & Tree         & Conflict   & Construction Site & Exchange   \\
S18         & Construction Site & Conflict   & Tree         & None    \\
S19         &              & Competiton &              & Cooperate  \\
S20         &              & Competiton &              & Conflict   \\
S21         &              & Competiton &              & Competiton \\
S22         &              & Competiton &              & Coercion   \\
S23         &              & Competiton &              & Exchange   \\
S24         &              & Competiton &              & None    \\
S25         & Construction Site & Coercion   & Tree         & Cooperate  \\
S26         & Tree         & Coercion   &              & Conflict   \\
S27         & Tree         & Coercion   &              & Competiton \\
S28         & Tree         & Coercion   &              & Coercion   \\
S29         & Construction Site & Coercion   &              & Exchange   \\
S30         & Tree         & Coercion   &              & None    \\
S31         & Construction Site & Exchange   &              & Cooperate  \\
S32         & Construction Site & Exchange   &              & Conflict   \\
S33         & Tree         & Exchange   &              & Competiton \\
S34         & Construction Site & Exchange   &              & Coercion   \\
S35         & Tree         & Exchange   & Construction Site & Exchange   \\
S36         & Construction Site & Exchange   &              & None    \\
S37         &              & None    & Tree         & Cooperate  \\
S38         &              & None    & Construction Site & Conflict   \\
S39         &              & None    & Tree         & Competiton \\
S40         &              & None    & Tree         & Coercion   \\
S41         &              & None    & Construction Site & Exchange   \\
S42         &              & None    & Construction Site & None    \\
S43         &              & Cooperate  & Construction Site & Cooperate  \\
S44         &              & Cooperate  &              & Conflict   \\
S45         &              & Cooperate  & Tree         & Competiton \\
S46         &              & Cooperate  & Construction Site & Coercion   \\
S47         &              & Cooperate  & Construction Site & Exchange   \\
S48         &              & Cooperate  & Construction Site & None    \\
S49         &              & Conflict   & Construction Site & Cooperate  \\
S50         &              & Conflict   &              & Conflict   \\
S51         &              & Conflict   &              & Competiton \\
S52         &              & Conflict   & Tree         & Coercion   \\
S53         &              & Conflict   &              & Exchange   \\
S54         &              & Conflict   &              & None    \\
S55         &              & Competiton &              & Cooperate  \\
S56         &              & Competiton &              & Conflict   \\
S57         &              & Competiton &              & Competiton \\
S58         &              & Competiton &              & Coercion   \\
S59         &              & Competiton &              & Exchange   \\
S60         &              & Competiton &              & None    \\
S61         &              & Coercion   &              & Cooperate  \\
S62         &              & Coercion   &              & Conflict   \\
S63         & Tree         & Coercion   & Tree         & Competiton \\
S64         &              & Coercion   &              & Coercion   \\
S65         &              & Coercion   &              & Exchange   \\
S66         &              & Coercion   &              & None    \\
S67         &              & Exchange   &              & Cooperate  \\
S68         &              & Exchange   &              & Conflict   \\
S69         &              & Exchange   &              & Competiton \\
S70         &              & Exchange   &              & Coercion   \\
S71         &              & Exchange   &              & Exchange   \\
S72         &              & Exchange   &              & None   
\end{longtable}

For each of the experiment scenario we show the Yellow robot's estimation of the physical and social goal of the red robot at each time step.
The overall performance of Social MDPs and the baselines against the ground truth is reported in \cref{fig:model-correlations}, with \cref{tab:goal_estimations_multiple_levels} showing the inferences of the model and baselines.

\begin{longtable}[c]{@{}c@{}c@{}c@{}}
\caption{Using Social MDP, at different levels of reasoning, Yellow robot estimates the physical and social goal of the red robot at each time step. For physical goal estimates, the lines in ({\red in red is tree},{\blue in blue is construction site} show the physical goal estimates at each time-step. At level one, an agent has a belief over the physical goal of another agent. Humans and models predict what this belief is (the degree to which the agent believes that the other agent is heading toward the tree or the construction site). For social goal estimates, the lines in ({\blue in blue is cooperate},{\olive in olive is conflict}, {\green in green is competition}, {\red in red is coercion}, {\yellow in yellow is exchange}) show the social goal estimates at each time-step. }
\label{tab:goal_estimations_multiple_levels}\\
Scenario Id &
  \begin{tabular}[c]{@{}c@{}}Physical goal estimation\\ (Level 1)\end{tabular} &
  \begin{tabular}[c]{@{}c@{}}Social goal estimation\\ (Level 2)\end{tabular} \\[2ex]
\endfirsthead
\endhead
\end{longtable}
